# Supplementary material for: An Optimization Algorithm for Customer Topological Paths Identification in Electrical Distribution Networks
Source: arXiv:2409.09073 source file (2024-09-09)
Supplement: Supplementary file 1 [file Appendix.tex]

% \subsection{Further explanation for first constraint}
% \label{appen:firstC}

\textcolor{blue}{What about dropping it? I think it does not add much.}

\ld{You need the A* algorithm, except if it is the same algorithm as the reference you will select.}

\subsection{Tree-search Algorithm}
\label{appen:Hpath}
Given the factorial term in Eq. \ref{eq:size_h} and its scalability challenges, a tree-search algorithm is employed to generate the set of hypothetical paths $\mathcal{H}$. \\
The tree-search algorithm, denoted as $CustomerPaths(\mathcal{E}, c, N)$, takes as input the set of elements $\mathcal{E}$, an element of type customer $c \in Subset(\mathcal{E}, customer)$, and a maximum number of paths $N$. It then outputs a set of paths, up to $N$, that are most likely to be the real paths for the customer $c$.\\
The algorithm starts by building a tree, where:
\begin{itemize}
    \item The root of the tree is the element of type $customer$ ($c$) under consideration.
    % \item according to the well-defined information $i'_2$ and $i'_3$, the leaf of the tree is the element of type $plug$ related to the customer (leaf $l=c.plug$)
    \item The intermediate nodes include elements that can be directly connected to the element $c$ according to the $Connections()$ function.
    % Moreover, they include also all the connections of these connected elements, up to the leaves of the tree.
    \item Two types of leaves exist:
        \begin{itemize}
            \item junction leaf: denoted as $l$, and it is the ending point of a path. According to the well-defined information $i'_3$.
            % the junction leaf is the element of type $junction$ related to the customer, $l=c.junction$
            \item dead-end leaf: is a leaf that has no other connection available.
        \end{itemize}
\end{itemize}
If two elements, $e_i,e_j \in \mathcal{E}$, are reachable, there is an edge between them. Each edge has a weight, that, initially, depends on the distance between the two elements it connects. Therefore:
\begin{align}
    w_{e_i \to e_{j}} = Dist(e_i, e_j)
\end{align}
where $w_{e_i \to e_{j}}$ represents the weight of the edge connecting the elements $e_i$ and $e_j$.\\
After the tree is built, the algorithm starts by finding some partial paths, $pp$. Each partial path represents a set containing the customer $c$ and some elements among its possible connections. \\
% and any reachable elements of its connections. \\
Each partial path has a cost. The cost of a partial path depends on the weights of the edges connecting its elements and the distance between the last element in the partial path and the leaf $l$, formally:
\begin{align}
\label{eq:costpath}
    cost_{pp} = \sum_{i}^{|pp|-1} w_{e_i \to e_{i+1}} + Dist(pp_{|pp|}, l)
\end{align}
with $w_{e_i \to e_{i+1}}$ the weight of the edge that connects the two elements, $e_i$ and $e_{i+1}$, and $pp_{|pp|}$ the last element of the partial path $pp$.\\
For example, a partial path composed by the customer, $c$, and one of its next connections, $e_{next}$, has a cost of:
\begin{align}
    cost = w_{c \to e_{next}} + Dist(e_{next}, l)
\end{align}
After identifying all the partial paths, the algorithm selects the one with the lowest cost. This selection enables the tree search to efficiently choose the sequence of elements that most quickly approaches the leaf $l$.
Afterward, the weights of the partial path edges are updated, multiplying them by a scaling factor $\alpha$, with $\alpha>1$. Increasing the weights of the edges is useful to prioritize the search of paths whose elements have not been explored yet.\\
The algorithm keeps iterating, therefore identifying longer partial paths, until:
\begin{itemize}
    \item the leaf, $l$, is reached,
    \item a dead-end is reached, there is no $e_{next}$ to consider,
    \item the length of the partial path is greater than the threshold $L$, according to the well-defined information $i'_4$.
\end{itemize}
The algorithm stops when all the paths have been considered or at least $N$ paths are found.

\subsection{Validity path constraint term}
\label{appen:1stconstraint}

Let us consider the example network shown in Fig. \ref{fig:1stconstraint}. In such a case, the set of elements $\mathcal{E}$ is given by 8 elements.

\begin{figure}[h]
\centering
\begin{subfigure}[b]{0.4\textwidth}
        \centering
        \includegraphics[width=\textwidth]{Images/1st constraint1.png}
        \caption{Acceptable solution}
        \label{fig:1st constraint1}
\end{subfigure}
\hfill
\begin{subfigure}[b]{0.4\textwidth}
        \centering
        \includegraphics[width=\textwidth]{Images/1st constraint2.png}
        \caption{Not acceptable solution}
        \label{fig:1st constraint2}
\end{subfigure}
\caption{Small network example to explain the validity path constraint in the optimization problem}
\label{fig:1stconstraint}
\end{figure}
\begin{align}
    \mathcal{E} = \{ e_1, e_2, e_3, e_4, e_5, e_6, e_7, e_8 \}
\end{align}
with their types: 
\begin{table}[H]
\centering
\caption{}
\label{tab:proof_op1}
\resizebox{0.8\columnwidth}{!}{%
\begin{tabular}{|c|c|}
\hline
\textbf{Subset}          & \textbf{Number of elements} \\ \hline
$Subset(\mathcal{E}, customer)$    & 2                           \\ \hline
$Subset(\mathcal{E}, line)$        & 3                           \\ \hline
$Subset(\mathcal{E}, junction)$    & 2                           \\ \hline
$Subset(\mathcal{E}, transformer)$ & 1                           \\ \hline
\end{tabular}%
}
\end{table}

Let's assume the set of hypothetical paths is given by only 4 paths:
\begin{table}[h]
\centering
\caption{}
\label{tab:proof_op2}
\resizebox{0.8\columnwidth}{!}{%
\begin{tabular}{|c|c|c|c|c|c|c|c|c|}
\hline
     & e_1 & e_2 & e_3 & e_4 & e_5 & e_5 & e_6 & e_7 \\ \hline
h_1 & 1     & 0    & 1     & 1    & 0    & 1     & 0    & 1    \\ \hline
h_2 & 1     & 0    & 1     & 1    & 0    & 0     & 1    & 1    \\ \hline
h_3 & 0     & 1    & 0     & 1    & 0    & 1     & 0    & 1    \\ \hline
h_4 & 0     & 1    & 0     & 0    & 1    & 0     & 0    & 1    \\ \hline
\end{tabular}%
}
\end{table}

Let us consider that the methodology is run, and the solution is given by the two matrices, the matrix $\hat{\mathbf{P}}$:
\begin{align}
    \hat{\mathbf{P}} \! =
    \begin{blockarray}{cccc}
      h_1 & \! h_2 & \! h_3 & \! h_4 \\
    \begin{block}{(cccc)}
      1 & \! 0 & \! 1 & \! 0 \nonumber
    \end{block} 
  \end{blockarray}
\end{align}

\noindent For the matrix $\mathbf{J}$, let us consider two possible cases:
\begin{itemize}
    \item The solution in Fig. \ref{fig:1st constraint1}. This solution satisfies the first constraint. \\
    In such case, the matrix $\mathbf{J}$ is:
    \begin{align}
    \label{eq:Jsol1}
        \mathbf{J} \! = \!\!
            \begin{blockarray}{cccc}
            & \! e_3 & \! e_4 & \! e_5 \\
            \begin{block}{c(ccc)}
            j_1 \;\; & \! 1 & \! 1 & \! 0 \\
            j_2 \;\; & \! 0 & \! 0 & \! 0 \\
            \end{block}
            \end{blockarray}
    \end{align}
    
    \item The solution in Fig. \ref{fig:1st constraint2}. This solution does not satisfy the first constraint. \\
    In such case, the matrix $\mathbf{J}$ is:
    \begin{align}
    \label{eq:Jsol1}
        \mathbf{J} \! = \!\!
            \begin{blockarray}{cccc}
            & \! e_3 & \! e_4 & \! e_5 \\
            \begin{block}{c(ccc)}
            j_1 \;\; & \! 0 & \! 1 & \! 0 \\
            j_2 \;\; & \! 1 & \! 0 & \! 0 \\
            \end{block}
            \end{blockarray}
    \end{align}
\end{itemize}

\noindent The constraint of interest states that all the elements of every path have to be assigned to the same feeder terminal junction. This is guaranteed when each element on the left side of the matrix is greater or equal to the element on the right side of Eq. \ref{eq:constraint1}. \\
Therefore, for the case shown in Fig. \ref{fig:1st constraint1} the result of the constraint would be: \ld{I think I would detail step by step eq 22b, so compute JxHr, then (JxHr).Ht and so on for one solution. It would help the reader if he does not have to do the calculations himself to be sure to understand.}
\begin{align}
\label{eq:Jsol1}
        \begin{blockarray}{ccccc}
        & \! h_3 & \! h_4 & \! h_5 & \! h_5 \\
        \begin{block}{c(cccc)}
        j_1 \;\; & \! 2 & \! 0 & \! 1 & \! 0 \\
        j_2 \;\; & \! 0 & \! 0 & \! 0 & \! 0 \\
        \end{block} 
        \end{blockarray}
        \; \geq
        \begin{blockarray}{ccccc}
        & \! h_3 & \! h_4 & \! h_5 & \! h_5 \\
        \begin{block}{c(cccc)}
        j_1 \;\; & \! 2 & \! 0 & \! 1 & \! 0 \\
        j_2 \;\; & \! 0 & \! 0 & \! 0 & \! 0 \\
        \end{block}
        \end{blockarray}
\end{align}
From Eq. \ref{eq:Jsol1} it is possible to see that the condition of great or equal is verified for each element.

While, for the case shown in Fig. \ref{fig:1st constraint2} the result of the first constraint would be:
\begin{align}
\label{eq:Jsol2}
        \begin{blockarray}{ccccc}
        & \! h_1 & \! h_2 & \! h_3 & \! h_4 \\
        \begin{block}{c(cccc)}
        j_1 \;\; & \! 1 & \! 0 & \! 0 & \! 0 \\
        j_2 \;\; & \! 0 & \! 1 & \! 0 & \! 0 \\
        \end{block} 
        \end{blockarray}
        \; \geq
        \begin{blockarray}{ccccc}
        & \! h_1 & \! h_2 & \! h_3 & \! h_4 \\
        \begin{block}{c(cccc)}
        j_1 \;\; & \! 2 & \! 0 & \! 1 & \! 0 \\
        j_2 \;\; & \! 0 & \! 0 & \! 0 & \! 0 \\
        \end{block}
        \end{blockarray}
\end{align}
From Eq. \ref{eq:Jsol2} it is possible to see that the condition of great or equal is not verified for each element. This is due to the fact that there exists (at least) a path that contains elements that belong to different feeder terminal junctions. For example, the hypothetical path $h_1$ is composed by the elements $\{ e_1, e_3, e_4, e_5, e_7 \}$ but the elements $e_3$ and $e_4$ belong to different feeder junctions, $j_1$ and $j_2$ respectively. Therefore, since the first constraint is not satisfied, the solution represented in Fig. \ref{fig:1st constraint2} is not acceptable.

% \newpage
% \[
% \textcolor{red}{\mathcal{A}},
% \mathcal{B},
% \mathcal{C},
% \mathcal{D},
% \textcolor{red}{\mathcal{E}},
% \textcolor{red}{\mathcal{F}},
% \mathcal{G},
% \mathcal{H},
% \textcolor{red}{\mathcal{I}},
% \textcolor{blue}{\mathcal{J}},
% \mathcal{K},
% \mathcal{L},
% \mathcal{M},
% \mathcal{N},
% \mathcal{O},
% \textcolor{red}{\mathcal{P}},
% \mathcal{Q},
% \mathcal{R},
% \mathcal{S},
% \textcolor{red}{\mathcal{T}},
% \mathcal{U},
% \mathcal{V},
% \mathcal{W},
% \mathcal{X},
% \mathcal{Y},
% \mathcal{Z}
% \]
